# Supplementary material for: Shallow Trap States Control Electrical Performance of Amorphous Oxide Semiconductor Thin-Film Transistors
Source: arXiv:2602.06329 ancillary file (2026-02-06)
Supplement: Supplementary file 1 [file supplement.pdf]

# Supplementary Information for: Shallow Trap States Control Electrical Performance of Amorphous Oxide Semiconductor Thin-Film Transistors

Måns J. Mattsson,[1] Jinhan Lee,[2] Christopher E. Malmberg,[3] Jared Parker,[1] Kyle T. Vogt,[1] Hyemi Kim,[4] Minji Hong,[4] Pilsang Yun,[4] Daewon Ha,[4] Taeyoon Lee,[2] Paul H.-Y. Cheong,[3] John F. Wager,[5] and Matt W. Graham[1,*]

[1]*Department of Physics, Oregon State University, Corvallis, OR, 97331-6507, USA*
[2]*School of Electrical and Electronic Engineering, Yonsei University, Seoul 03722, Korea*
[3]*Department of Chemistry, Oregon State University, Corvallis, Oregon 97331-4003, USA*
[4]*Advanced Device Research Lab, Samsung Electronics, Hwaseong-si, Gyeonggi-do, 18448, Korea*
[5]*School of Electrical Engineering and Computer Science, Oregon State University, Corvallis, OR, 97331-5501, USA*

## S1. TFT DEVICE PREPARATION

Three types of a-IGZO TFTs are used in this study: (1) backgated TFTs with systematic In-enrichment, (2) nanoscale dimension topgated TFTs for DRAM application developments, and (3) backgated TFTs with designs appropriate for display panel applications.

For TFTs with systematic In-enrichment, highly boron-doped p-type silicon (p++) substrates with a 100 nm thermally grown $SiO_2$ layer were used as the gate platform for TFT fabrication. Prior to device processing, the substrates were sequentially cleaned by ultrasonication in acetone, isopropyl alcohol, and deionized water for 5 min each. In-rich amorphous indium–gallium–zinc oxide (a-IGZO) thin films were deposited at room temperature by radio frequency (RF) magnetron sputtering under a working pressure of ∼15 mTorr, using an $Ar/O_2$ mixed-gas plasma. The Ar flow rate was fixed at 50 sccm, while the oxygen flow ratio, defined as $R_{O_2}$=[$O_2$ ]/([Ar]+[$O_2$ ]), was systematically adjusted depending on the deposition conditions. [1] For the fabrication of In-rich a-IGZO TFTs with a channel thickness of 15 nm, the channel layers were formed by RF–RF co-sputtering from a-IGZO and $In_2O_3$ targets, enabling precise modulation of the indium content. To suppress plasma coupling effects arising from the simultaneous operation of two RF power sources at identical frequencies, a CEX mode was employed, with the operating frequencies of the individual generators appropriately offset. The RF power applied to the a-IGZO target was fixed at 120 W, whereas the $In_2O_3$ target power was varied between 20 and 100 W to tune the indium concentration in the channel layer. Concurrently, $R_{O_2}$was adjusted to approximately 2, 6, 9, 12, and 15% to regulate the density of oxygen vacancies in the In-rich a-IGZO films. Source and drain electrodes consisting of 40 nm-thick Al were deposited by thermal evaporation through a metal shadow mask. The devices were fabricated with channel lengths of 50, 100, 150, 200, and 250 $\mu$m and a fixed channel width of 1000 $\mu$m, corresponding to width-to-length ratios (W/L) of 20, 10, 6.67, 5, and 4, respectively.

The nanoscale top-gated a-IGZO TFTs for DRAM application developments were deposited on a silicon substrate with active channel dimensions of 140 nm width, 110 nm length, and 10 nm thickness. To study how the subgap DoS evolves under varying processing conditions, the a-IGZO growth conditions, annealing time, annealing environment, and channel thickness were systematically varied. The relative variation of processing conditions of these TFTs are summarized in Table S1. Two different growth methods were applied, labeled A and B. The post-deposition annealing time was varied across six different durations, labeled (#)1–6, with 1 being the shortest and 6 the longest. The annealing environment was varied using three different conditions, labeled A-C. For the device in Table S1 with line color red, an additional pre-treatment process was added prior to a-IGZO deposition.

The backgated display TFTs were deposited with a-IGZO channel dimensions of 4 $\mu$m width and 5 $\mu$m length. Table S2 summarizes the various processing conditions of the TFTs relative to the point-of-reference (POR) device by different source-drain sputtering techniques, oxygen partial pressure during deposition, and channel composition. In Table S2, oxalic acid refers to a combined wet and dry etching process. Low damage 1 and 2 refers to different dry etching methods. TATM refers to an additional layer of Mo on top of the POR Ti/Al/Ti source-drain contacts. $PO_2$ 80% refers to the oxygen partial pressure during deposition, compared to $PO_2$ 20% for POR. CAAC refers to c-axis-aligned crystalline active channel. Additional TFTs with a top-gated structure were also compared.

* Corresponding author: graham@physics.oregonstate.edu

| Line Color | Growth Condition | Anneal Time (#) | Anneal Environment | Channel Thickness (nm) |
|---|---|---|---|---|
| Black | A | 6 | A | 10 |
| Green | A | 3 | B | 10 |
| Purple | A | 2 | B | 10 |
| Orange | A | 1 | B | 10 |
| Yellow | B | 6 | C | 10 |
| Blue | B | 4 | A | 10 |
| Red | B | 4 | C | 10 |
| - | B | 5 | C | 5 |
| - | B | 4 | C | 10 |

TABLE S1. Relative processing conditions for 9 topgated nanoscale a-IGZO TFTs for DRAM development applications displayed in Figure 3.

| Line Color | $V_O$ Peak Density $\times 10^{11}$ ($cm^{-2}eV^{-1}$) | S.S (mV/dec) | Mobility, $\mu_{EKV}$ ($cm^2\ V^{-1}\ s^{-1}$) | Simulated $W_{TA}$ (meV) | Processing Condition |
|---|---|---|---|---|---|
| - | 2.0 | 109 | 6.9 | 27 | Oxalic Acid |
| Black | 2.2 | 126 | 8.0 | 23 | Low Damage 1 |
| Purple | 2.8 | 165 | 6.3 | 26 | Low Damage 2 |
| Red | 3 | 161 | 5.7 | 28 | TATM |
| - | 3.1 | 160 | 5.9 | 26 | POR |
| Orange | 3.5 | 170 | 4.9 | 30 | $PO_2$ 80% |
| Yellow | 5.1 | 238 | 3.9 | 31 | CAAC |

TABLE S2. Electrical characteristics and processing conditions for 7 backgated display panel a-IGZO TFTs displayed in Figure 6.

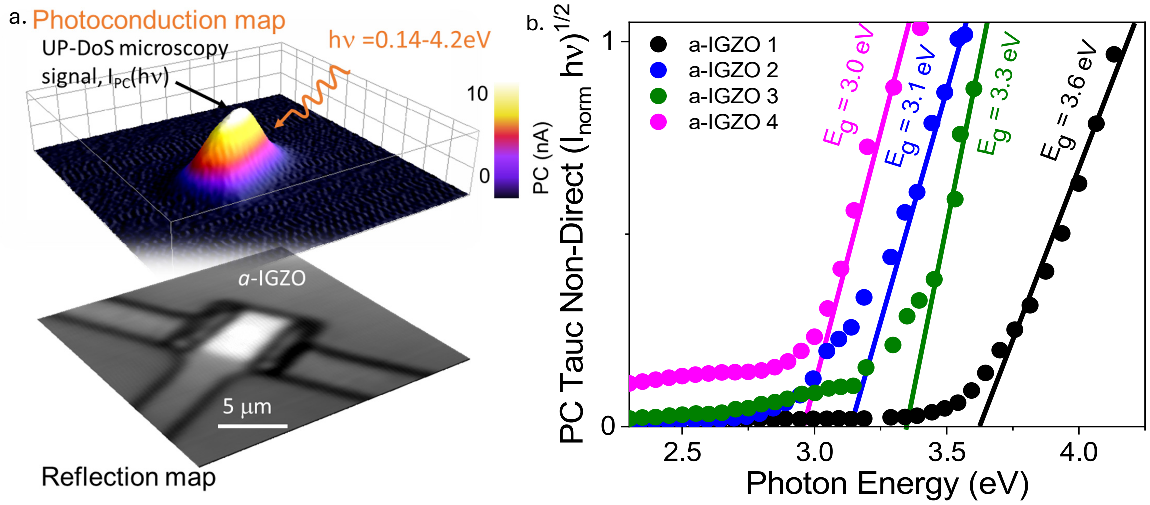


..

FIG. S1. (a) UP-DoS is a microscopy method where the active TFT channel photoconduction is resolved spatially and spectrally. (b) Non-direct Tauc scaling of photoconduction enables bandgap extraction for different a-IGZO TFTs.

## S2. UP-DOS PHOTOCONDUCTION SPECTUM ANALYSIS AND BANDGAP EXTRACTION

Similar to optical absorption, when the photon energy, $h\nu > E_g$, the measured TFT photoconduction spectrum $I_{PC}(h\nu)$ is approximately proportional to the joint density of states (JDoS) as $I_{PC}(h\nu) \propto \int_{-\infty}^{\infty} g_{VB}(E-h\nu)g_{CB}(E)dE$. Here, the electrons are promoted from the filled valence band DoS, $g_{VB}$ to the empty conduction band DoS, $g_{CB}$. Alternatively, when $h\nu < E_g$ the sub-bandgap laser energies generate a photoresponse is instead approximately the

integrated subgap DoS, or $I_{PC}(h\nu) \propto \int_{-h\nu}^{0}(E)g(E)dE$. Here, the subgap DoS $g(E)$ is small compared to the empty conduction band DoS, $g_{CB}(E)$. Under these conditions for the UP-DoS TFT microscopy, our tunable lasers excites trapped electrons from any filled subgap defect state within $h\nu$ of the conduction band minimum (CBM). As a result, the TFT photoconduction increases by an amount proportional to the photon energy integrated trap density or $N_{tot}(h\nu) = \int_{-h\nu}^{0} g(E)dE$. As this study concerns amorphous n-type TFTs, initial subgap defect wavefuctions should be localized in real space, and the amorphous-nature relaxes most optical absorption selection rules.

To analyze the near-band-gap behavior of the UP-DoS TFT photoconduction spectrum, we adopt the Tauc and Urbach band-tail state analyses, which are conventionally applied to optical absorption spectra.[2] To make this connection, we approximate that the induced photocurrent as proportional to the photons absorbed $I_{PC} \propto N_{tot}(h\nu)(1-e^{-\alpha l})$, where $\alpha$ is the absorption coefficient, and $l$ is the TFT charge accumulation region thickness. Under the good approximation that the TFT charge accumulation layer thickness, $l$ is always much smaller than optical skin depth $\delta = 1/\alpha$, the TFT photoresponse is well approximated as $I_{PC} \propto N_{tot}(h\nu)\alpha l$. This end-form is essentially identical to that expected from the optical absorption response, allowing standard Tauc and Urbach scaling to be applied to UP-DoS acquired data on TFTs.[3]

Over the 30+ different a-IGZO TFTs investigated here, the extracted Tauc bandgaps ranged from 3.0 eV to 3.6 eV depending on the specific processing conditions of the a-IGZO active channel. Figure S1 shows photoconduction converted to a Tauc non-direct extraction plot for 4 representative a-IGZO TFTs. Otherwise, for each of the roughly monotonically decreasing steps observed in the $I_{PC}$ subgap spectrum, data analysis of the raw UP-DoS photoconduction spectrum proceeds by fitting the entire subgap response to a sequence of error (erf) functions. The mathematical expression for fitting to each subgap defect step observed in $I_{PC}$ is:

$$I_{PC}(h\nu) \propto \int_{-h\nu}^{E_{CBM}=0} g(E)dE \tag{S1}$$

$$\approx \sum_i A_i(1 + \mathrm{erf}[w_i(h\nu - E_{o,i})]) \tag{S2}$$

where $A_i$ are the function amplitudes, $w_i$ are the step-widths, and $E_{o,i}$ are each of the sequential defect step (peak) energies. The derivative with energy of the above function recovers the Gaussian peak lineshape, and recovers the final subgap DoS in a-IGZO TFTs from the raw UP-DoS TFT photoconduction spectrum. Only the subgap peak amplitudes, $A_i$ and energies, $E_{o,i}$ are free-fit parameters. The peak widths, $w_i$ are roughly constant for oxygen vacancies, suggesting similar environmental broadening due to the amorphous nature of the lattice.

## S3. DFT+U SIMULATION SUPPLEMENTAL INFORMATION

The twenty formula unit (140 atoms) cells were taken through melt and quench molecular dynamics simulation via the General Lattice Utility Program (GULP), and then melted to 4000 K for 30 ps and subsequently cooled by 100 K/ps until the system reached 300 K, where the cell was equilibrated for 3 ps. [4] The resulting structures were refined using Vienna ab initio Simulation Package (VASP) and using the Perdew-Burke-Ernzerhof (PBE) generalized gradient approximation (GGA) functional theory. [5–9] Using the conjugate gradient algorithm, three individual relaxations were done using a 1 × 1 × 1 k-point mesh centered at the gamma point. Ions are only allowed to relax for the first and third relaxation, and the second relaxation only allows a change in cell size. All density of states calculations were done using GGA + U with a 4 × 4 × 4 Monkhorst Pack k-point mesh. The In-4d, Ga-3d, and Zn-3d U values of 7, 8, and 8 were extracted from Noh et al.[10] The O-2p U value of 7 was extracted from Ma et al. [11]

In order to compare DFT+U defect calculations with experimentally measured DoS in Figs. 7-8, the DFT+U must be corrected for the underestimated bandgap. Preserving the relative distance of defect peaks to the band edges, the correction is by a weighted scissoring method, where peaks closer to CBM get increasingly shifted to a higher energy according to, $E_{new} = -(\frac{E_{g,exp}}{E_{g,DFT}}E_{org} - E_{exp})$ where $E_{new}$ is the new peak energy of the scissored peak referenced (CBM=0), $E_{org}$ is the original DFT+U calculated peak energy (VBM=0), $E_{g,exp}$ is the experimental direct bandgap of the specific TFT and $E_{g,DFT} = 1.6$ eV is the DFT+U calculated bandgap. Lastly, all 80 DFT+U DoS simulations are superimposed on the UP-DoS to identify which oxygen vacancy coordinations dominate experimentally. While multiple assignments are possible in the congested midgap region, only 4 shallow distinct peaks are simulated within ∼0.4 eV of conduction band minima.

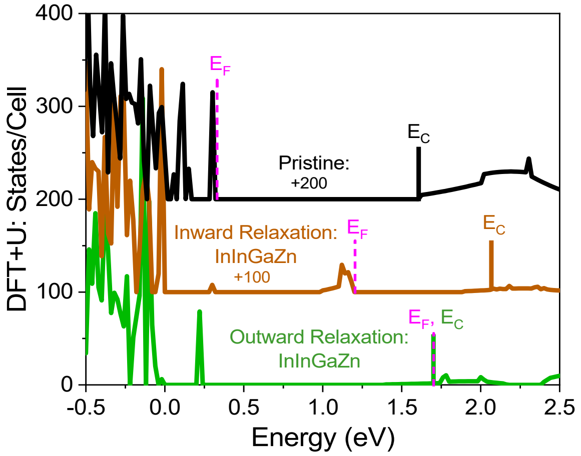


FIG. S2. DFT+U–simulated density of states for three representative unit cells: pristine (no oxygen vacancy, black), an InInGaZn coordinated oxygen vacancy with inward relaxation of neighboring atoms (brown), and an InInGaZn coordinated oxygen vacancy with outward relaxation of neighboring atoms (green). For all simulated unit cells with outward relaxation of neighboring atoms, no new oxygen vacancy state appears within the bandgap. Instead, the defect state appears above the conduction band minimum, and the Fermi level appears at the conduction band minimum.

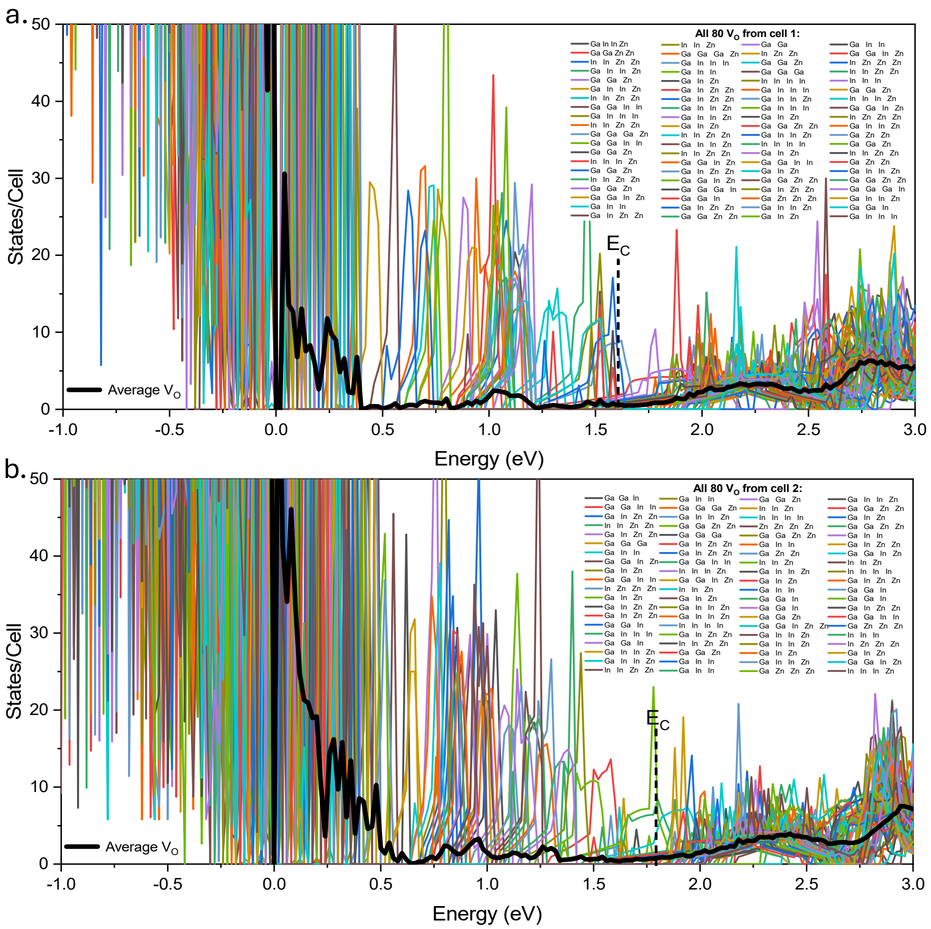


FIG. S3. Compendium of two different DFT+U–simulated density of states from two different amorphous cell structures. Panels a and b correspond to the two different cell structures and each contains 80 curves resulting from the introduction of a single oxygen vacancy. By comparing the pattern of repeated peak energies, local coordination environments can be inferred (see Table S3 below). The black curve plot is the mean result.

| Number # | Peak Energy eV | Density $\times 10^{16}$cm$^{-3}$ | $V_O$ cation coordination |
|---|---|---|---|
| 0 | 0.12 | 2.0 | **InInInGa, InInGaZn, InInZ, InInZnZn** |
| 1 | 0.32 | 9.7 | **InGaGa**, InInZn |
| 2 | 0.60 | 4.8 | **InInZnZn, InInGaZn, InInGaGa**, GaGaZn |
| 3 | 0.92 | 0.9 | **GaGaZn, GaGaGaIn, GaInZn, InZnZnZn**, InInIn |
| 4 | 1.25 | 4.0 | **InInGaZn, InInZnZn**, GaInZn, GaZnZnZn |
| 5 | 1.47 | 26 | **InInGaGa, InInGa, InInZn, InInGaZn**, GaGaIn, GaInZnZn, GaGaZnZn, GaGaInZn, GaInZn |
| 6 | 1.86 | 66 | **GaGaZn, GaGa,GaGaIn, GaGaInZn**, GaInIn |
| 7 | 2.05 | 18 | InGaZn, GaGaInZn, GaGaIn |
| 8 | 2.33 | 270 | **GaGaGaZn, GaGaInZn, GaGaZnZn,InGaZnZn, InZnZnZn**, GaInIn |
| 9 | 2.70 | 210 | **InInGaZn**, GaInZn, GaGaZn |
| 10 | 3.03 | 27 | InZnZn, GaGaIn, GaZnZnZn |

TABLE S3. UP-DoS measured peak energy (CBM = 0), density, and all possible DFT+U metal-oxygen vacancy coordination environments for all experimentally observed peaks 0-10. Coordination environments suggested by experimental data from In-enrichement are highlighted in bold.

## S4. UP-DOS EXPERIMENTAL EXTRA INFORMATION

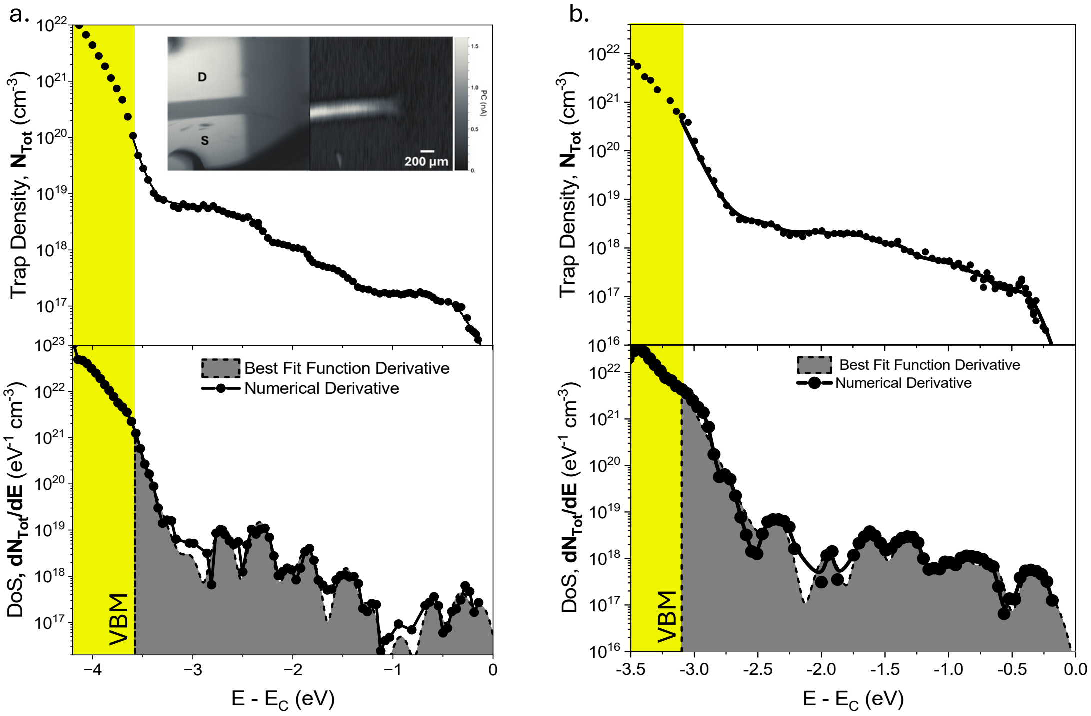


FIG. S4. (a,b) UP-DoS analysis for two different a-IGZO TFTs. Upper panels plot the raw UP-DoS data and the corresponding best fit functions, while lower panels show the extracted density of states obtained from the analytical (filled gray) and numerical (black dots) derivatives. Upper panel insets display back-reflection and photoconduction scanning maps of each TFT under near-bandgap excitation.

Figure S5a and b provides a comparison between the numerical derivative with minimal smoothing beforehand and the analytical derivative approach in two different a-IGZO TFTs. The two approaches yield largely the same DoS. However, the analytical approach of taking derivatives of the best-fit error functions yields improved signal-to-noise and enables deconvolution of individual defect peaks.

For select TFTs, such as the nanoscale examples shown in Figure 3, a power saturation measurement to find the absolute scaling constant $k_0$ was not possible. The device architecture in the nanoscale devices do not permit near bandgap excitation of the active channel due to the top-gated structure and a silicon substrate. In these cases, the absolute DoS was rescaled by a general factor $k_0 \approx 0.3$ W/eV while preserving the relative differences in the DoS

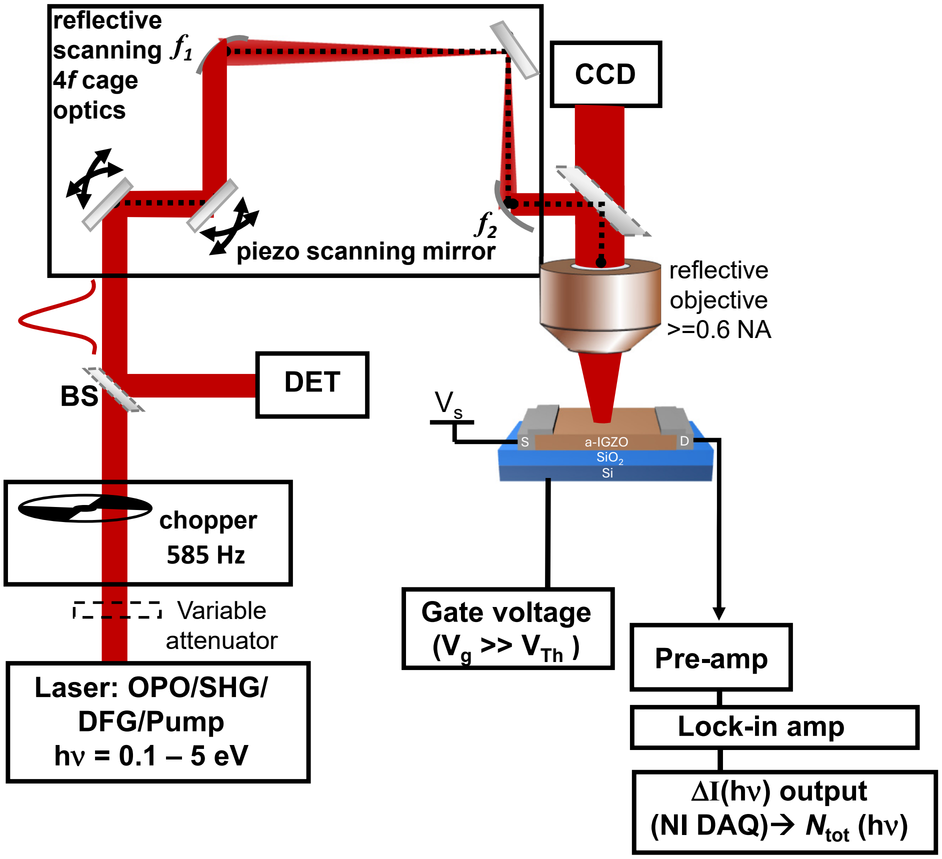


FIG. S5. The generalized homebuilt UP-DoS experimental schematic.[12] The laser wavelength is tuned from the UV to the mid-IR to selectively excite filled defect states to the conduction band directly in the TFT active channel, and the resulting photoconduction is recorded using lock-in detection.

between individual TFTs.

As high-energy photons can induce instabilities and stress effects in a-IGZO,[13–15] UP-DoS is always performed by scanning from low to high photon energies. Transfer curves are taken before and after each UP-DoS spectrum, with no noticeable change induced by the measurement.

## S5. SHALLOW TRAP CORRELATIONS WITH TFT PERFORMANCE METRICS

This section provides the additional details that clarify the mobility and subthreshold swing (S.S.) trends shown in Figure 2a and b. EKV mobility, $\mu_{EKV}$, strongly varies with the density of electrons induced into the active channel, and is thus strongly gate voltage dependent. Out of the 15 display TFTs considered in Figure 2a, there are two subsets with different gate oxide capacitance values. In order to accurately compare $\mu_{EKV}$ across TFTs with different gate oxide capacitance, each $\mu_{EKV}$ value is extracted at the same gate induced carrier density satisfying the charge sheet equation $C_{ox}(V_G\text{-}V_{ON})/q = 5 \times 10^{11}$ cm$^{-2}$. Figure 2b fits this extracted $\mu_{EKV}$ to the expected red line shown, which scales inversely with shallow trap density according to the drift mobility equation [16, 17]

$$\mu = \mu_o \left( \frac{n}{n + n_T} \right) \tag{S3}$$

where $\mu_o$ is the trap-free mobility of an electron, n is the number of free electrons, and $n_T$ is the number of electrons occupying a trap state. A best fit of Equation S3 suggests a trap free mobility of $\mu_0 \approx 23$ cm$^2$V$^{-1}$s$^{-1}$ consistent with the $\mu_o = 22$ cm$^2$V$^{-1}$s$^{-1}$ as the typical reported value for amorphous transport in $In_1Ga_1Zn_1O_x$. [17–20] Figure S2 presents the same analysis as above applied to the nanoscale DRAM TFTs, with the exception that all TFTs have the same gate oxide capacitance. The mobilities of these TFTs are significantly lower than those of conventional a-IGZO

devices due to increased series resistance as the channel dimensions are reduced. As shown in Figure S6a, the trap density is extracted at 0.7 eV from the conduction band mobility edge in each TFT. The EKV mobility is extracted at a gate overvoltage of 2V, as displayed in Figure S6b. Then, Figure S6c plots the two TFT metrics, revealing a strong correlation between mobility and trap density.

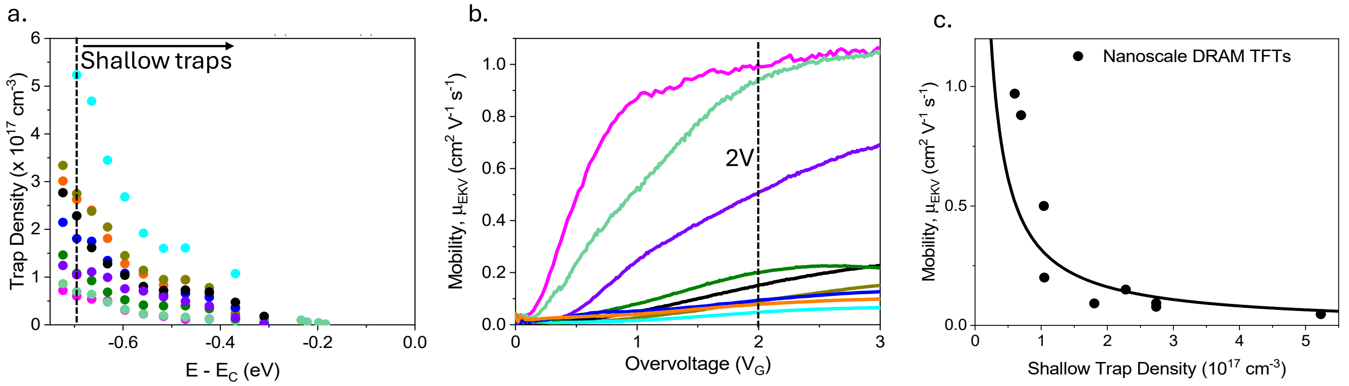


FIG. S6. **(a)** Shallow trap density measured by UP-DoS in 9 different nanoscale a-IGZO TFTs with various processing conditions. **(b)** The EKV mobility curves extracted directly from each respective TFT transfer curve. **(c)** EKV mobility plotted as a function of measured shallow trap density for each TFT device.

For the subthreshold swing and trap density correlation plot shown in Figure 2c, the same display and nanoscale TFTs as previously discussed were used. The subthreshold swing is expected to be related to the gate oxide capacitance and the trap density, as described in the equation: [21]

$$\text{S.S.} = \frac{kT}{q} \ln 10 \left( 1 + \frac{qD_{it}}{C_{ox}} \right) \tag{S4}$$

where T is the temperature, $D_{it}$ is the interfacial trap density and $C_{ox}$ is the gate oxide capacitance. To correct for the two different values of oxide capacitance in the different display TFTs, the subthreshold swing of one subset is adjusted as:

$$\text{S.S}_{\text{corr}} = \left( \text{S.S} - \frac{kT}{q} \ln 10 \right) \frac{C_{OX_1}}{C_{OX_2}} + \frac{kT}{q} \ln 10 \tag{S5}$$

where $C_{OX_1}$ and $C_{OX_2}$ are the two gate oxide capacitances of the two subsets. Note the fundamental thermionic limit is $\frac{kT}{q} \ln 10$ and is readily seen in all S.S. fits to data in Fig. 2b. This equation enables a direct comparison of the trap-induced contribution to the subthreshold swing across the two subsets of devices with different gate oxide capacitance.

## S6. SIMULATED TRANSFER CURVES: VARYING PEAK ENERGY AND WIDTH

Figure S7a, b and c presents the simulated TFT gate induced trap density, drift mobility, and transfer curve with shifting Gaussian peak energy of only the most dominant trap state. This trap state is observed by UP-DoS to lie 0.33 eV below the conduction-band mobility edge. As expected, the gate-induced trap density shown in Figure S7a is effectively constant as the total shallow trap density is not varied. However, a small change in effective shallow trap density was observed in the most shifted simulation (0.13 eV, yellow), as a small portion of the peak is now buried beneath the conduction band tail and is no longer relevant to device operations. Figure S7c shows that for any variation of the peak energy, a significant distortion occurs in the transfer curve relative to its original shape.

Figure S7d, e, and f show how the simulated TFT gate induced trap density, drift mobility, and transfer curve vary with shifting Gaussian widths. All Gaussian peaks are varied from a standard deviation of $\sigma = 30$ meV to $\sigma = 140$ meV, while preserving the total integrated trap density by correspondingly adjusting the Gaussian peak densities. Similarly to above, the most significant change is observed in the distortion of the transfer curves as observed in Figure S7f. Together, Figure S7f and c, and the previous result of Figure 5, show how the transfer curve shape on a logarithmic scale is strongly governed by the specific subgap density of states. The Gaussian peak energies, widths, and amplitudes are all essential parameters for accurately modeling TFT transfer curves. This result also highlights the excellent agreement between the simulated and experimental transfer curves when using the UP-DoS-derived Gaussian parameters (red curves), which are required to reproduce the experimental data.

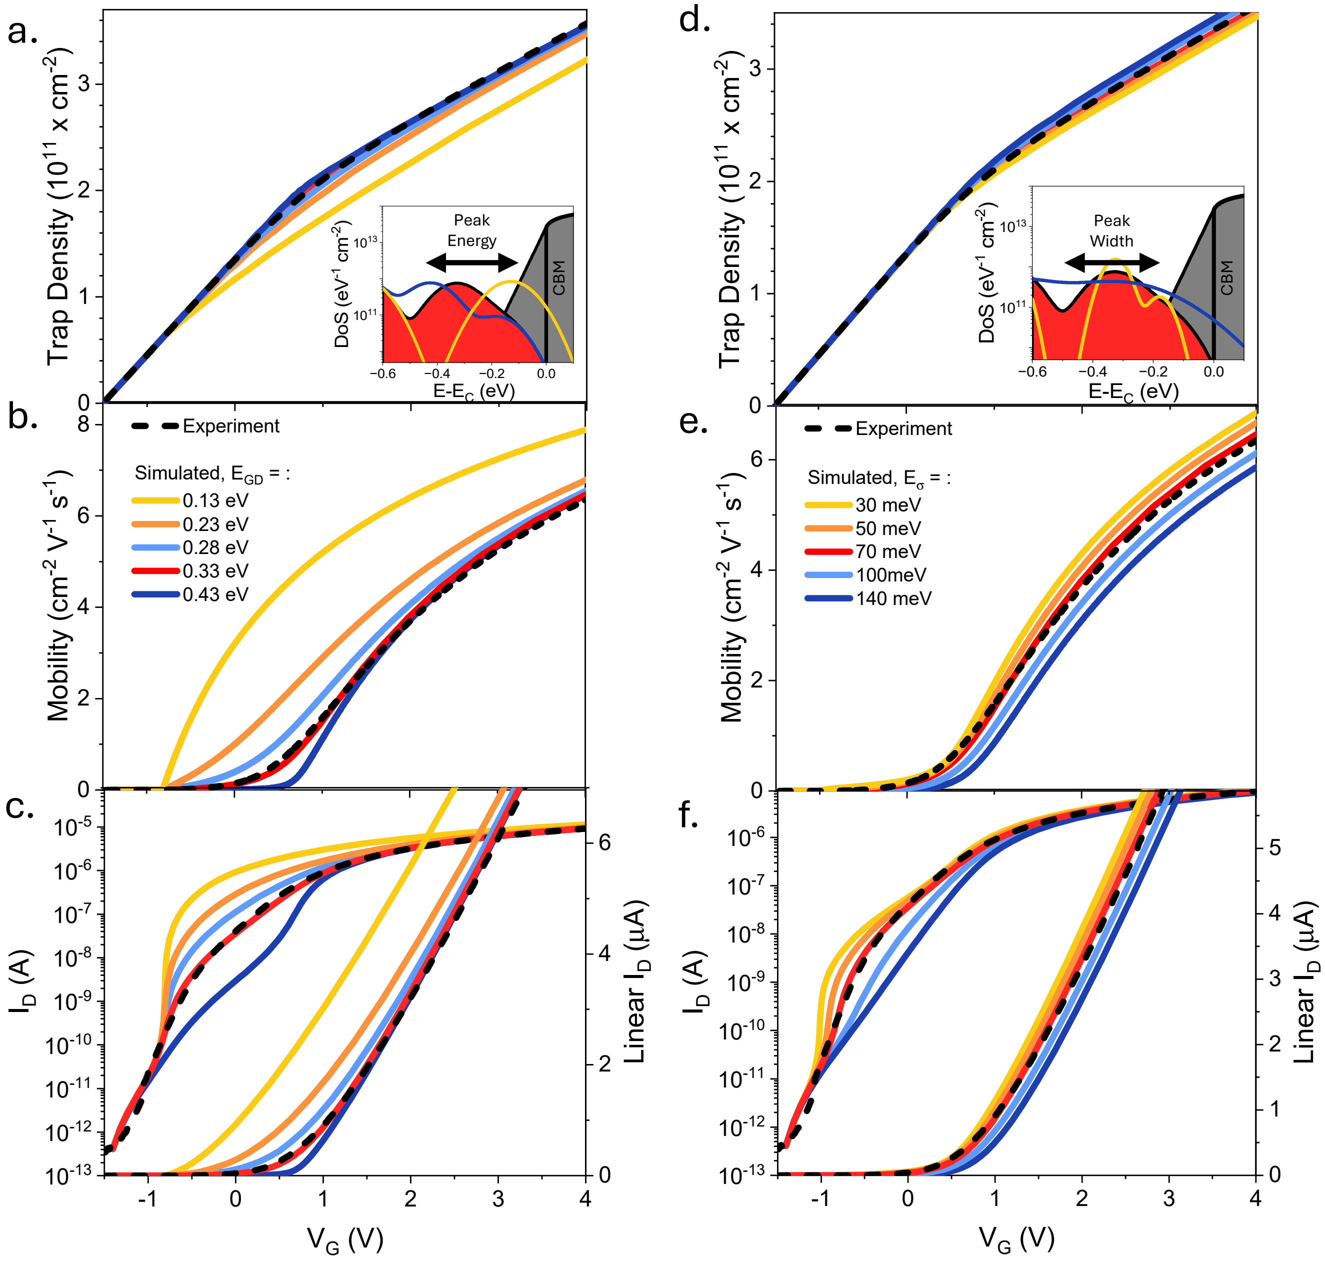


FIG. S7. DoS simulated TFT **(a)** gate induced trap density, **(b)** drift mobility and **(c)** transfer curve with varying Gaussian peak energy of the most dominant trap state. The peak is experimentally observed at 0.33 eV from the conduction band mobility edge. DoS Simulated TFT **(d)** gate induced trap density, **(e)** drift mobility and **(f)** transfer curve when varying all Gaussian peak widths while conserving the total shallow trap density.

## S7. TFT TRANSFER SIMULATION EQUATIONS FROM EXPERIMENTAL UP-DOS

The three shallow defect peaks (peak numbers 0, 1, 2) as measured by UP-DoS are put into to the TFT simulation in a Gaussian form:

$$g_{SD}(E) = A \exp\left[-\frac{(E-E_0)^2}{2\sigma^2}\right] \ (\mathrm{cm^{-2}\,eV^{-1}}) \tag{S6}$$

where A, $\sigma$ and $E_0$ are the Gaussian parameters determined experimentally by UP-DoS. The conduction band tail state is modeled as an decreasing exponential function: [17]

$$N_{TA} = \frac{1}{2\pi^2}\left(\frac{2m^*}{\hbar^2}\right)^{3/2}\sqrt{\frac{W_{TA}}{2}}e^{\frac{E-E_{CME}}{W_{TA}}}\ (\mathrm{cm}^{-3}\,\mathrm{eV}^{-1}) \tag{S7}$$

where $W_{TA}$ is the conduction band Urbach energy and $m^* = 0.34\ m_0$ is the a-IGZO electron effective mass. The conduction band states are modeled using the equation: [17]

$$g_C(E) = \frac{1}{2\pi^2}\left(\frac{2m^*}{\hbar^2}\right)^{3/2}\sqrt{E-E_C}\ (\mathrm{cm}^{-3}\,\mathrm{eV}^{-1}) \tag{S8}$$

To ensure continuity between the acceptor tail states and the extended conduction band states, the conduction band mobility edge energy, $E_{CME}$, is defined as: [17]

$$E_{CME} - E_C = \frac{W_{TA}}{2} \tag{S9}$$

For any given Fermi energy, each individual DoS is numerically evaluated using the Fermi-Dirac occupation function: [17]

$$n = \int_{-\infty}^{\infty} g_C(E)\, f_{FD}(E, F_n)\, dE \tag{S10}$$

$$f_{FD}(E, F_n) = \frac{1}{1+e^{\frac{E-F_N}{k_b T}}} \tag{S11}$$

where $F_N$ is the electron quasi-Fermi energy level. The charge density is then simply calculated by $Q = n \times q$, where q is the charge of the electron. As the simulation is operating under a charge sheet approximation, the volumetric charge densities retrieved from inputting Equations S7 and S8 into Equation S10 is converted to a charge sheet density by $Q_{2D} = Q_{3D}^{2/3}$.[17]

The free charge density, $Q = n_C \times q$, is due to an electron occupying a state in the conduction band. The trapped charge density, $Q_T = n_{TA} \times q + n_{SD} \times q$, is the summation of the total occupation of Gaussian shallow donor states and exponential acceptor tail states. Now, the fraction of free charge density relative to total charge density ($Q + Q_T$) can be evaluated as a function of the quasi-Fermi energy level, and can be expressed as an effective TFT drift mobility by Equation 2. Finally, by invoking the charge sheet approximation, the quasi-Fermi energy level can be directly mapped to an applied gate overvoltage axis by Equation 3 and subsequently be compared to experimental data.

Only the gate induced trapped charge density is relevant to TFT operations. To account for already filled trapped states before the TFT turns on, the calculated $Q_T$ for when $V_G = V_{ON}$ is subtracted from the total $Q_T$ density. This subtraction ensures that deep states do not directly impact TFT transfer curve.

The fixed simulated parameters (non-adjustable) are as follows: T = 293 K (room temperature), $C_{ox}$ (determined by specific TFT structure), $m^* = 0.34\ m_0$ (material specific), $V_{ON}$ (measured device parameter), the quasi-Fermi energy for when $V_G = V_{ON}$ ($E_F \approx$ -0.65 eV) determined by Equation 6, and the experimental UP-DoS observed Gaussian parameters (A, $E_0$, $\sigma$). However, the absolute scaling of the UP-DoS measured DoS is initially treated as a free parameter, but is kept constant between devices and individual defect peak amplitudes. The only adjustable parameter applied in the simulation between different TFTs is the conduction band Urbach energy, $W_{TA}$ = 20-31 meV, which defines the slope of the linear operating regime in the transfer curve.

## S8. TFT SIMULATION WITH NO ADJUSTABLE FREE PARAMETERS

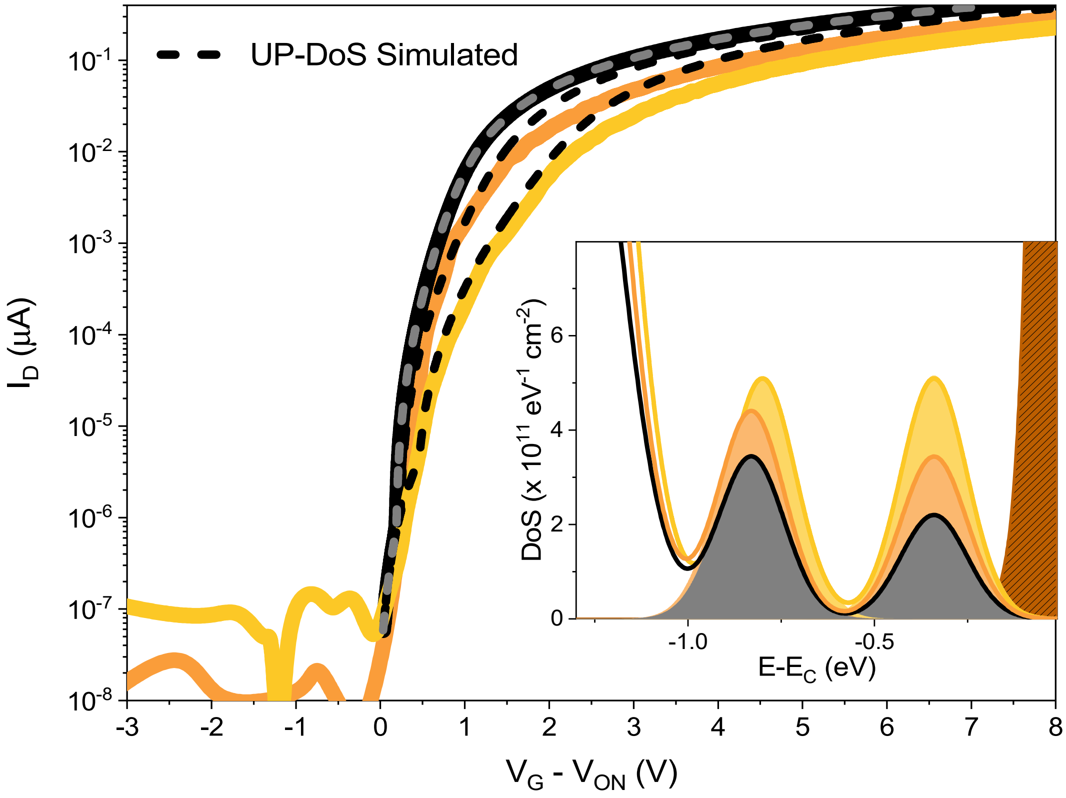


FIG. S8. Three TFT transfer curves processed under different conditions (colored lines). Dashed lines show simulated transfer curves generated directly from the UP-DoS–measured defect peaks, using a fixed conduction band tail Urbach energy and no adjustable parameters. The simulations show excellent agreement in the subthreshold region but deviate from the experimental data above threshold. The inset shows the experimentally measured subgap density of states used to generate each simulated curve.

## S9. TEMPERATURE DEPENDENCE OF TFT TRANSFER SIMULATION

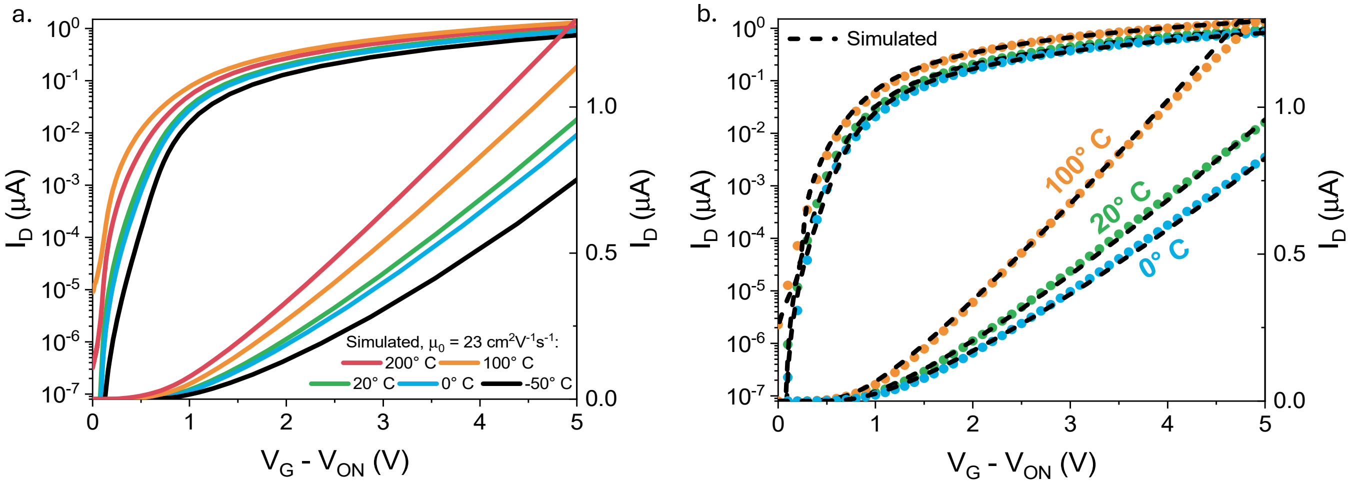


FIG. S9. **(a)** Simulated transfer curves for varying simulation temperatures using a constant $\mu_0$ parameter. **(b)** Three experimental TFT transfer curves of the same device taken at 0°, 20° and 100° C (red, green and blue dots). Dashed lines show simulated transfer curves for each respective temperature.

Figure S9a presents the DoS simulated curves for varying input temperatures, -50° C to 200°. The population of electrons in extended conduction band states for each quasi-Fermi level energy increases with temperature, resulting in a higher drift mobility and corresponding drain current. However, this effect is only partially responsible for the real experimental temperature dependence of transfer curves. The extended state trap-free mobility, $\mu_0$, is known to also increase as a function of operating temperature. This thermal activation of $\mu_0$ is well reported in literature and is expected due to the diffusive nature of electron mobility in amorphous oxide semiconductors. [17, 22] Figure S9b shows experimental (colored dots) and DoS simulated transfer curves (dashed lines) for three different operating temperatures: 0°, 20°, and 100° C. The trap free mobility simulation parameter, $\mu_0$, necessary to fit experimental data increases from $\mu_0 = 21$ at 0° C, to $\mu_0 = 23$ at 20° C and finally to $\mu_0 = 26$ $cm^2V^{-1}s^{-1}$ at 0° C.

---

[1] S. Lee, J. Lee, M. Lee, D. K. Lee, Y. Han, G. C. Park, J. S. Park, S. Lee, J. H. Cho, I. Yun, *et al.*, High-performance oxide semiconductor tft with a-igzo/in-rich a-igzo heterostructure using quantum confinement effects: Enhancing mobility and reliability, Journal of Alloys and Compounds , 182035 (2025).
[2] J. Klein, L. Kampermann, B. Mockenhaupt, M. Behrens, J. Strunk, and G. Bacher, Limitations of the tauc plot method, Advanced Functional Materials **33**, 2304523 (2023).
[3] M. J. Mattsson, K. M. Niang, J. Parker, D. J. Meeth, J. F. Wager, A. J. Flewitt, and M. W. Graham, Defect density of states of tin oxide and copper oxide p-type thin-film transistors, Advanced Electronic Materials , 2400929 (2025).
[4] J. D. Gale, J. Chem. Soc., Faraday Trans. **93**, 629 (1997).
[5] G. Kresse and J. Furthmüller, Efficiency of ab-initio total energy calculations for metals and semiconductors using a plane-wave basis set, Computational materials science **6**, 15 (1996).
[6] G. Kresse and J. Furthmüller, Efficient iterative schemes for ab initio total-energy calculations using a plane-wave basis set, Physical review B **54**, 11169 (1996).
[7] G. Kresse and D. Joubert, From ultrasoft pseudopotentials to the projector augmented-wave method, Physical review b **59**, 1758 (1999).
[8] J. P. Perdew, K. Burke, and M. Ernzerhof, Generalized gradient approximation made simple, Physical review letters **77**, 3865 (1996).
[9] G. Kresse and J. Hafner, Ab initio hellmann-feynman molecular dynamics for liquid metals, Journal of non-crystalline solids **156**, 956 (1993).
[10] H.-K. Noh, K. J. Chang, B. Ryu, and W.-J. Lee, Electronic structure of oxygen-vacancy defects in amorphous in-ga-zn-o semiconductors, Phys. Rev. B **84**, 115205 (2011).
[11] X. Ma, Y. Wu, Y. Lv, and Y. Zhu, Correlation effects on lattice relaxation and electronic structure of zno within the gga+u formalism, The Journal of Physical Chemistry C **117**, 26029 (2013).
[12] K. T. Vogt, M. Mattsson, and M. W. Graham, Ultrabroadband photoconduction method and apparatus for defect density

of states microscopy in semiconductor devices, US Patent Application US2025102448A1 (2025), filed by Oregon State University. United States Patent and Trademark Office.

[13] R. Nakazawa, A. Matsuzaki, K. Shimizu, I. Nakamura, E. Kawashima, S. Makita, K. Tanaka, S. Yasuno, H. Sato, H. Yoshida, *et al.*, Reliable measurement of the density of states including occupied in-gap states of an amorphous in–ga–zn–o thin film via photoemission spectroscopies: Direct observation of light-induced in-gap states, Journal of Applied Physics **135** (2024).

[14] J. Robertson and Y. Guo, Light induced instability mechanism in amorphous ingazn oxide semiconductors, Applied Physics Letters **104** (2014).

[15] M. Mativenga, F. Haque, M. M. Billah, and J. G. Um, Origin of light instability in amorphous igzo thin-film transistors and its suppression, Scientific reports **11**, 14618 (2021).

[16] A. Nenashev, J. Oelerich, S. Greiner, A. Dvurechenskii, F. Gebhard, and S. Baranovskii, Percolation description of charge transport in amorphous oxide semiconductors, Physical Review B **100**, 125202 (2019).

[17] J. F. Wager, Amorphous semiconductor mobility physics and tft modeling, Amorphous Oxide Semiconductors: IGZO and Related Materials for Display and Memory , 105 (2022).

[18] I. I. Fishchuk, A. Kadashchuk, A. Bhoolokam, A. de Jamblinne de Meux, G. Pourtois, M. Gavrilyuk, A. Köhler, H. Bässler, P. Heremans, and J. Genoe, Interplay between hopping and band transport in high-mobility disordered semiconductors at large carrier concentrations: The case of the amorphous oxide ingazno, Physical Review B **93**, 195204 (2016).

[19] K. A. Stewart, B.-S. Yeh, and J. F. Wager, Amorphous semiconductor mobility limits, Journal of Non-Crystalline Solids **432**, 196 (2016).

[20] K. A. Stewart and J. F. Wager, Thin-film transistor mobility limits considerations, Journal of the Society for Information Display **24**, 386 (2016).

[21] J.-S. Lyu, A new method for extracting interface trap density in short-channel mosfets from substrate-bias-dependent subthreshold slopes, ETRI Journal **15**, 11 (1993).

[22] P.-Y. Liao, T.-C. Chang, T.-Y. Hsieh, M.-Y. Tsai, B.-W. Chen, Y.-H. Tu, A.-K. Chu, C.-H. Chou, and J.-F. Chang, Investigation of carrier transport behavior in amorphous indium–gallium–zinc oxide thin film transistors, Japanese Journal of Applied Physics **54**, 094101 (2015).
